# Supplementary material for: Realization of high-fidelity unitary operations on up to 64 frequency bins
Source: arXiv:2206.06059 source file (2024-02-15)
Supplement: Supplementary file 1 [file Frequency_bin_unitaries_supplement.pdf]

# Realization of high-fidelity unitary operations on up to 64 frequency bins: Supplemental Material

Syamsundar De,<sup>1,2</sup> Vahid Ansari,<sup>1,3</sup> Jan Sperling,<sup>4</sup> Sonja Barkhofen,<sup>1</sup> Benjamin Brecht,<sup>1,\*</sup> and Christine Silberhorn<sup>1</sup>

<sup>1</sup>*Integrated Quantum Optics Group, Institute for Photonic Quantum Systems (PhoQS),  
Paderborn University, 33098 Paderborn, Germany*

<sup>2</sup>*Advanced Technology Development Centre, IIT Kharagpur, Kharagpur 721302, India*

<sup>3</sup>*E. L. Ginzton Laboratory, Stanford University, 348 Via Pueblo Mall, Stanford, California 94305, USA*

<sup>4</sup>*Theoretical Quantum Science, Institute for Photonic Quantum Systems (PhoQS),  
Paderborn University, 33098 Paderborn, Germany*

(Dated: February 15, 2024)

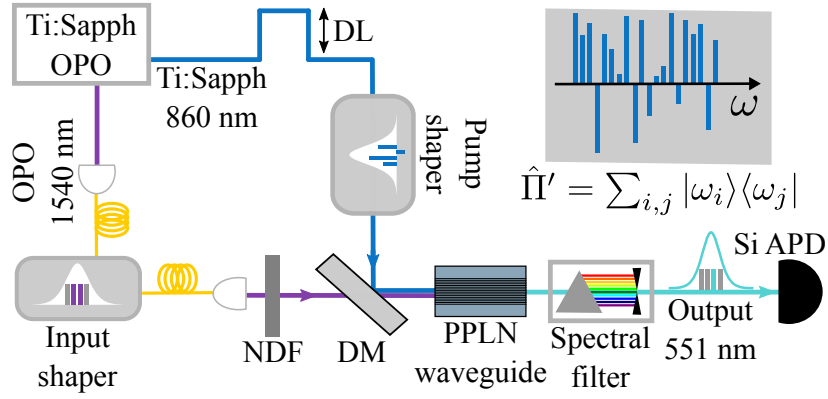

FIG. S1. Schematic of the setup. For details, please see the text.

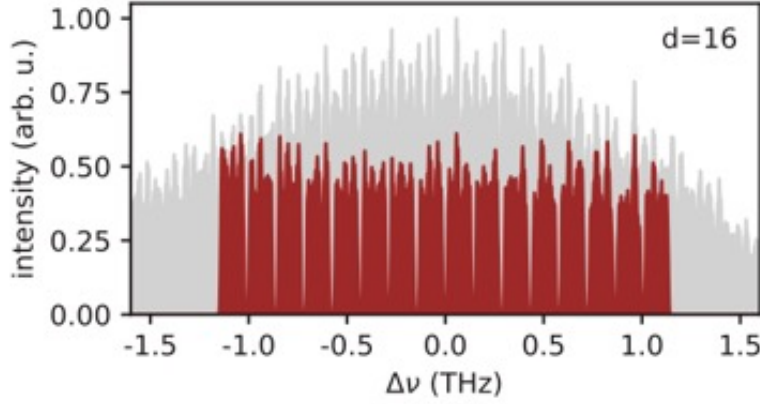

FIG. S2. Example of a shaped pump spectrum, where the initial spectrum (grey) has been equalized to yield 16 FBs with the same energy content (red). In this case, the bins have been carved from the centre of the pump pulse and have a width of approximately 100 GHz. Oscillations are caused by the limited resolution and discretization of the spectrometer used to measure the spectrum.

## DETAILS OF THE EXPERIMENTAL SETUP

We reproduced the sketch of the experimental setup from the main text in Fig. S1. We use a commercial titanium sapphire oscillator/optical parametric amplifier (Ti:Sapph/OPO) system that generates mode-locked pulse trains with pulse durations around 150 fs, corresponding to a spectral intensity FWHM of around 2.8 THz. The OPO pulses with a central wavelength of 1540 nm serve as input states  $|\psi\rangle$  for our measurements, while the Ti:Sapph pulses with a central wavelength of 860 nm are the pump pulses for the quantum pulse gate (QPG), which define the rotated projections  $\hat{\Pi}'$ . The OPO pulses are attenuated and coupled to a single mode fibre, before propagating through a commercial pulse shaper. After shaping, they are attenuated to the single photon level using a series of neutral density filters (NDF). The Ti:Sapph pulses' timing is adjusted with a delay line (DL) and the pulses are subsequently sent to a homebuilt pulse shaper based on a  $4f$ -line and a spatial light modulator. The resolutions of the pulse shapers are 10 GHz for the OPO and 20 GHz for the Ti:Sapph, respectively. Based on these numbers, we chose a frequency bin (FB) width of 40 GHz with guard bands of 36 GHz between bins. This leads to a total spectral span of 4.0 THz for the maximum number of 64 FBs, close to the full  $1/e^2$ -width of the pulse spectrum. When shaping the pump spectrum into 64 FBs, special care has been taken to equalize the amplitudes of all bins before applying the shaping. Otherwise, the FBs close to the central wavelength would contain significantly more energy than the FBs at the edges, which would result in low projection fidelities.

An example for this is shown in Fig. S2. Note that the bin width is around 100 GHz in this case and we only carve 16 bins

from the centre of the pulse. After the equalization of the individual FBs, the shaping would be applied. One schematic example for a pump shape is given in the inset of Fig. S1. We note that the exact shape of the pump, in particular the phases of the individual FBs, can be set arbitrarily and are dictated by the target unitary. When shaping the maximum of 64 FBs, the resulting overall energy of the pump pulse reduced to 0.125 pJ as an effect of bin equalization and shaping.

After the shaping, we spatially overlap the Ti:Sapph and OPO pulses on a dichroic mirror (DM) and couple them into a periodically poled lithium niobate (PPLN) waveguide, which we fabricated in house. The waveguide has a length of 35 mm and a poling period of  $\Lambda = 4.4 \mu\text{m}$ . Individual mode-matching telescopes for the two beams are not shown. The PPLN waveguide is the quantum pulse gate (QPG), in which a dispersion-engineered sum-frequency generation takes place. Due to the limited pump pulse energy, the conversion efficiency of the QPG was limited to 0.1 %.

We separate the converted output light at 551 nm from the remaining pump and input light with another DM (not shown) before sending it to a  $4f$ -line for spectral filtering. The  $4f$ -line is based on gratings and an adjustable slit and serves to filter out the side lobes of the phase matching function of the QPG. We set a filter bandwidth of 50 GHz, which optimizes projection fidelities while still transmitting most of the converted light. After the spectral filter, we couple the transmitted light to a single-mode fibre (not shown) and count photons with a silicon avalanche photo diode in Geiger mode (SiAPD). Counts are recorded on a time tagger and stored on a computer (not shown).

### QPG OPERATION PRINCIPLE

In the following, we briefly summarise the operation principle of the QPG. On the logical level, a QPG implements a beam splitter operating on programmable temporal modes of light described by the following operator transformations

$$\hat{A} \mapsto \cos(\theta)\hat{A} + \sin(\theta)\hat{C}, \quad (1)$$

$$\hat{C} \mapsto \cos(\theta)\hat{C} - \sin(\theta)\hat{A}. \quad (2)$$

Here,  $\hat{A}$  is the programmable input temporal mode. In our experiment,  $\hat{A} = \sum_j c_j \hat{f}_j$ , where  $\hat{f}_j$  describes the  $j$ -th FB and the  $c_j$  are complex coefficients.  $\hat{C}$  is the output mode. We have already said that the QPG is based on dispersion-engineered sum-frequency generation. If the spatial and polarization modes of all involved fields are fixed—this is the case when using a periodically poled waveguide—we can describe the QPG interaction by the following Hamiltonian:

$$\hat{H}_{QPG} = \theta \int d\omega_{\text{in}} d\omega_{\text{out}} G(\omega_{\text{in}}, \omega_{\text{out}}) \hat{a}(\omega_{\text{in}}) \hat{c}^\dagger(\omega_{\text{out}}) + \text{h.c.} \quad (3)$$

Here,  $\theta$  collects all constants and  $G(\omega_{\text{in}}, \omega_{\text{out}}) = \alpha(\omega_{\text{out}} - \omega_{\text{in}}) \phi(\omega_{\text{in}}, \omega_{\text{out}})$  is the so-called transfer function that maps input to output frequencies and which itself is a product of the pump function  $\alpha(\omega_{\text{out}} - \omega_{\text{in}})$  and the phase matching function  $\phi(\omega_{\text{in}}, \omega_{\text{out}})$ . Due to the dispersion engineering, the group velocities of pump and input are matched. In addition, the QPG is operated such that the total pump bandwidth is larger than the phase matching bandwidth. In this case, the transfer function becomes separable and can be written as

$$G(\omega_{\text{in}}, \omega_{\text{out}}) = f(\omega_{\text{in}}) \times g(\omega_{\text{out}}), \quad (4)$$

where  $f(\omega_{\text{in}}) = \alpha(\Omega_{\text{out}} - \omega_{\text{in}})$  is defined by the complex spectrum of the pump and  $g(\omega_{\text{out}}) = \phi(\omega_{\text{out}})$  is the phase matching, which is independent of  $\omega_{\text{in}}$ , and  $\Omega_{\text{out}}$  is the central frequency of the converted output light. Using this, we can write

$$\hat{H}_{QPG} = \theta \int d\omega_{\text{in}} f(\omega_{\text{in}}) \hat{a}(\omega_{\text{in}}) \int d\omega_{\text{out}} g(\omega_{\text{out}}) \hat{c}^\dagger(\omega_{\text{out}}) + \text{h.c.} = \theta \hat{A} \hat{C}^\dagger + \text{h.c.}, \quad (5)$$

where we have defined broadband creation and annihilation operators  $\hat{A}$  and  $\hat{C}^\dagger$ . We identify this Hamiltonian with a special quantum mechanical beam splitter that acts on temporal modes. In particular, an input mode that is defined by the complex spectrum of a classical pump pulse is transferred into an output mode, while all other modes are transmitted. The conversion efficiency  $\eta$  of the QPG is then proportional to the field overlap between the QPG input mode defined by the pump and the mode of the input state:

$$\eta \propto \int d\omega_{\text{in}} \alpha^*((\Omega_{\text{out}} - \Omega_{\text{pump}}) - \omega_{\text{in}}) \psi(\omega_{\text{in}}), \quad (6)$$

with  $\psi(\omega_{\text{in}})$  the temporal mode of the input state  $|\psi\rangle$ . Note that we have shifted the pump function to be centred at the central input frequency  $\Omega_{\text{in}} = \Omega_{\text{out}} - \Omega_{\text{pump}}$  with  $\Omega_{\text{pump}}$  the central pump frequency.

## PROGRAMMING UNITARIES AND PROJECTIONS

We said in the main manuscript that probabilities  $\{p\}$  associated with our measurement outcomes were given according to Born's rule as

$$p = \langle \psi | \hat{\Pi}' | \psi \rangle = \langle \psi | \hat{U}^\dagger \hat{\Pi} \hat{U} | \psi \rangle. \quad (7)$$

Here,  $\hat{\Pi}$  is the projection onto the original basis elements, while the matrix  $\hat{U}^\dagger$  encodes a basis rotation from the original basis to the new measurement basis. The columns of  $\hat{U}^\dagger$  contain the complex coefficients of the new measurement vectors. If we assume a FB basis with  $f_i(\omega_{\text{in}})$  the  $i$ -th FB and a unitary matrix  $\hat{U}$  that describes an  $N \times N$  optical network, we find that, in order to measure the  $j$ -th output mode of the network, we have to shape our pump according to

$$\alpha_j(\Omega_{\text{out}} - \omega_{\text{in}}) = \sum_{i=1}^N \hat{U}_{ij}^\dagger f_i(\omega_{\text{in}}). \quad (8)$$

If we count converted photons at the output of the QPG when applying this pump, we realize the projection  $\hat{\Pi}'_i$  that is associated with measuring the  $i$ -th output of the unitary. In this way, we can project onto an arbitrary output of an arbitrary unitary. The standard measurement recipe will then follow along these steps:

1. Calculate the desired unitary operation  $\hat{U}$ .
2. Retrieve the associated pump shapes, which are encoded in the columns of  $\hat{U}^\dagger$ .
3. Set the first pump shape  $\alpha_1(\Omega_{\text{out}} - \omega_{\text{in}})$  and count photons for a predetermined time.
4. Continue to set the remaining  $N-1$  pump shapes and count photons for the same amount of time.
5. Retrieve the output probabilities from the measurements.
6. Choose a new unitary operation and go back to step 1.

All that remains now is to understand how to translate a given quantum walk (QW) unitary to our FB encoding.

## MAPPING QUANTUM WALK UNITARIES TO FREQUENCY BINS

We explain the mapping using the example of a Hadamard walk on a line. In this case, the coin space is two-dimensional,  $d_c = 2$ . Consequently, the coin operation  $\hat{C}_n$  is a  $2 \times 2$  unitary. In particular, the coin operation is the same at every single position of every step and is given by a Hadamard transformation of the form

$$\hat{H}_{\text{Had}} = \frac{1}{\sqrt{2}} \begin{pmatrix} 1 & 1 \\ 1 & -1 \end{pmatrix}. \quad (9)$$

This turns a coin state into a superposition and can, for example, be realized with a half-wave plate under an angle of  $22.5^\circ$  if the coin degree of freedom is encoded in polarization. The step operator is given by

$$\hat{S} = |0\rangle_c \langle 0|_c \otimes \sum_x |x+1\rangle \langle x| + |1\rangle_c \langle 1|_c \otimes \sum_x |x-1\rangle \langle x| \quad (10)$$

that is, depending on the coin state the walker takes a step to the left or to the right.

Let us now present an explicit example for the first step of a Hadamard walk on a line. In the first step, the walker will propagate from position 0—its initial position—to the positions +1 and -1, depending on the coin state. Hence we have a three-dimensional position space,  $d_x = 3$ , and a total system dimension of  $d = 3 \cdot 2 = 6$ . This means that we require six FBs  $f_1(\omega_{\text{in}}), \dots, f_6(\omega_{\text{in}})$ . FBs one and two encode position  $x = -1$ , FBs three and four encode position  $x = 0$ , and FBs five and six encode position  $x = +1$ . With this, we write the step operator as

$$\hat{S} = \begin{pmatrix} & x=-1 & x=0 & x=+1 \\ x=-1 & \begin{pmatrix} 0 & 0 \\ 0 & 0 \end{pmatrix} & \begin{pmatrix} 0 & 1 \\ 0 & 0 \end{pmatrix} & \begin{pmatrix} 0 & 0 \\ 0 & 0 \end{pmatrix} \\ x=0 & \begin{pmatrix} 0 & 0 \\ 1 & 0 \end{pmatrix} & \begin{pmatrix} 0 & 0 \\ 0 & 0 \end{pmatrix} & \begin{pmatrix} 0 & 1 \\ 0 & 0 \end{pmatrix} \\ x=+1 & \begin{pmatrix} 0 & 0 \\ 0 & 0 \end{pmatrix} & \begin{pmatrix} 0 & 0 \\ 1 & 0 \end{pmatrix} & \begin{pmatrix} 0 & 0 \\ 0 & 0 \end{pmatrix} \end{pmatrix}. \quad (11)$$

Here, the rows and columns encode the positions -1, 0, and +1, and the individual  $2 \times 2$  matrices account for the two-dimensional coin space. The corresponding coin operator is given by

$$\hat{C} = \hat{H}_{\text{Had}} \otimes \hat{f}_3 = \frac{1}{\sqrt{2}} \begin{pmatrix} 1 & 1 & 0 & 0 \\ -1 & 1 & 0 & 0 \\ 0 & 1 & 1 & 0 \\ 0 & 0 & -1 & 1 \end{pmatrix}. \quad (12)$$

Consequently, the unitary matrix describing the one step of the Hadamard walk on the is written as

$$\hat{U} = \hat{S}\hat{C} = \frac{1}{\sqrt{2}} \begin{pmatrix} 0 & 0 & -1 & 1 & 0 & 0 \\ 0 & 0 & 0 & 0 & 0 & 0 \\ 0 & 0 & 0 & 0 & -1 & 1 \\ 1 & 1 & 0 & 0 & 0 & 0 \\ 0 & 0 & 0 & 0 & 0 & 0 \\ 0 & 0 & 1 & 1 & 0 & 0 \end{pmatrix} \quad (13)$$

We remember that the columns of  $\hat{U}^\dagger$  encode the measurement modes  $\alpha_j(\Omega_{\text{out}} - \omega_{\text{in}})$ . Since, for this example,  $\hat{U}$  is real-valued, we find the measurement modes as the rows of  $\hat{U}$ . From this we obtain the following measurement modes:

$$\alpha_1(\Omega_{\text{out}} - \omega_{\text{in}}) = \frac{1}{\sqrt{2}} (-f_3(\omega_{\text{in}}) + f_4(\omega_{\text{in}})), \quad (14)$$

$$\alpha_2(\Omega_{\text{out}} - \omega_{\text{in}}) = 0, \quad (15)$$

$$\alpha_3(\Omega_{\text{out}} - \omega_{\text{in}}) = \frac{1}{\sqrt{2}} (-f_5(\omega_{\text{in}}) + f_6(\omega_{\text{in}})), \quad (16)$$

$$\alpha_4(\Omega_{\text{out}} - \omega_{\text{in}}) = \frac{1}{\sqrt{2}} (f_1(\omega_{\text{in}}) + f_2(\omega_{\text{in}})), \quad (17)$$

$$\alpha_5(\Omega_{\text{out}} - \omega_{\text{in}}) = 0, \quad (18)$$

$$\alpha_6(\Omega_{\text{out}} - \omega_{\text{in}}) = \frac{1}{\sqrt{2}} (f_3(\omega_{\text{in}}) + f_4(\omega_{\text{in}})). \quad (19)$$

If we now assume an input state

$$|\psi\rangle = (0, 0, 1, 0, 0, 0)^T, \quad (20)$$

which is localized at the input with a coin state pointing in one direction, we obtain a set of probabilities  $\{p\}$  that depend on the set of pump shapes  $\{\alpha_j\}$

$$\{p\} = |\langle \psi | \{\alpha_j\} \rangle|^2 = \{1/2, 0, 0, 0, 0, 1/2\}. \quad (21)$$

This is exactly the result we would get from evolving  $|\psi\rangle$  via  $\hat{U}$  and measuring in the original FB basis.

Although this is a simple example, it summarises the steps required to implement our approach. In principle, we can realize any unitary (and even non-unitary linear) operation. All that needs to be done is to adjust the FB superposition of the pump accordingly. A change of system dimension just means shaping more or less pump FBs, no overhaul of the experimental hardware is required.

Fig. S3 shows the implementation of the unitary associated with a Hadamard walk on a line with up to 15 steps, which is a direct extension of the above example. Note that for 15 steps, we already hit a system dimension of  $d = 62$ , close to our limit of  $d \leq 64$ . From a first glance we see that the experimental and theoretical positions distributions (Fig. S3(a) and (b), respectively) are very similar. This is corroborated by the calculated similarities, shown in Fig. S3(c). Finally, in Fig. S3(d), we plot the coin-resolved probability distribution for the 15-th step. The two colours mark the two coin states, error bars are shown in black and indicate statistical errors. Solid and empty bars indicate measurement and theory, respectively. Again, we find a very satisfying agreement between measurement and theory.

This shows that we have a) understood how to map a unitary to FBs, b) correctly shaped our pump modes, and c) realised a working experimental system with very good performance.

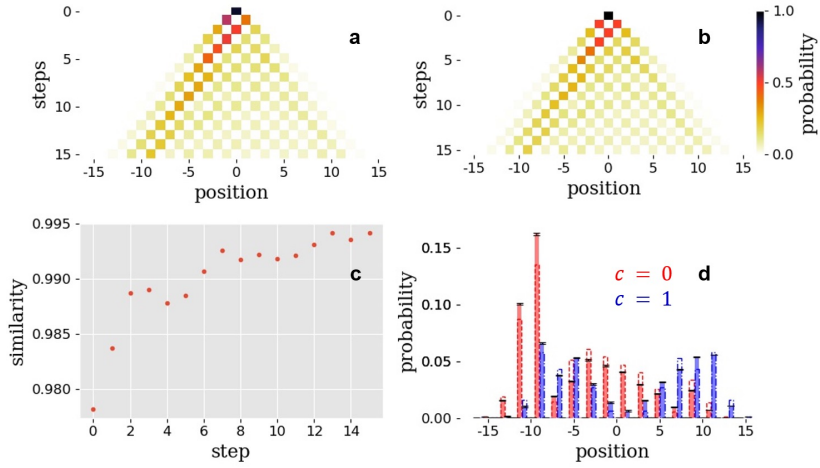

FIG. S3. Implementation of a unitary matrix associated with a Hadamard QW on a line over 15 steps. (a) Measured position distribution  $P(\vec{x})$ . (b) Theoretical position distribution. (c) Step-wise similarities between measurement and experiment. (d) Comparison between the measured and theoretical coin-resolved probability distributions (red, coin state  $c = 0$ ; blue, coin state  $c = 1$ ). Error bars (black) are statistical errors.

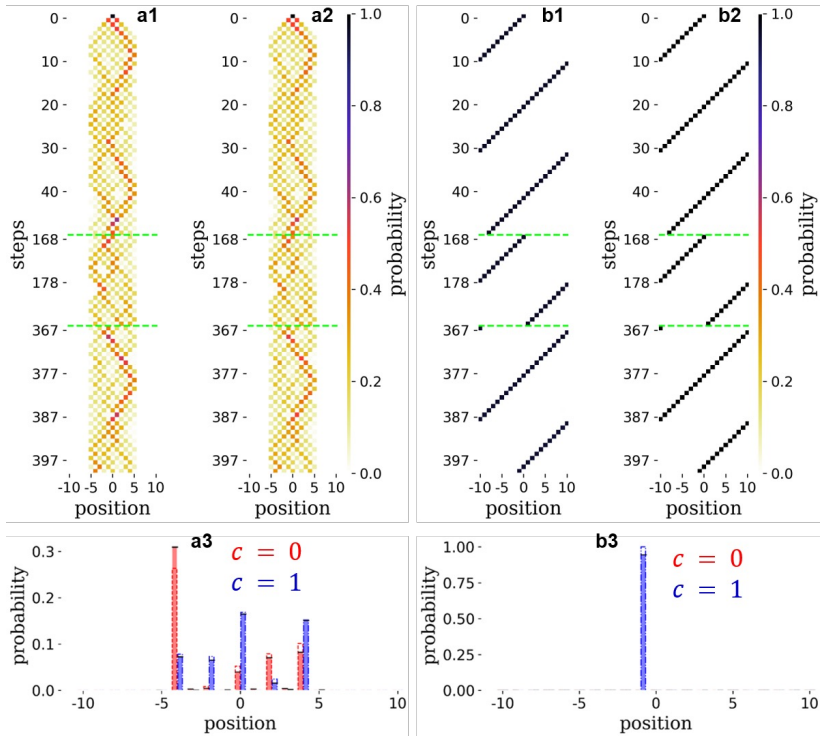

FIG. S4. Additional bounded QW unitaries. (a) Hadamard walk on a line with reflecting boundary conditions at positions  $\vec{x} = \pm 5$ . (b) Non-interacting walk with periodic boundary conditions at positions  $\vec{x} = \pm 10$ . For more information, see the text.

## ADDITIONAL MEASUREMENTS

In this section, we present additional measurements that add detail to the results presented in the main manuscript.

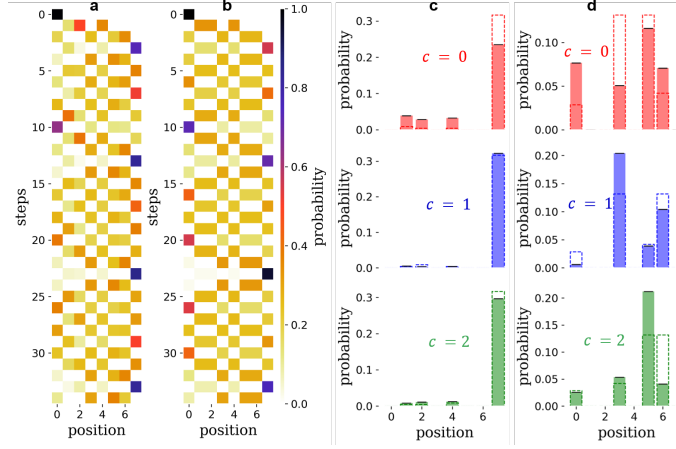

FIG. S5. Unitaries associated with a Grover walk on a cube. This is a three-dimensional version of the Grover walk on a hypercube shown in the main manuscript. (a) Experimental position distribution. (b) Theoretical position distribution. (c) Coin-resolved probability distribution for the 23rd step. (d) Coin-resolved probability distribution for the 34th step. For more information, see the text.

### Bounded quantum walks on a line

In Fig. S4, we investigated more bounded QWs that is, QWs on a finite graph. For all measurements, we input state is  $|\psi\rangle = |\vec{x}=0\rangle \otimes |c=0\rangle$  that is, a state that is localized at the origin with the coin state pointing in one direction. Note that this is the same state as above. Fig. S4(a) shows a Hadamard walk on a line with reflecting boundary conditions at positions  $\vec{x} = \pm 5$ . These are realized by implementing a reflection coin  $\hat{C}_R = \begin{pmatrix} 0 & 1 \\ 1 & 0 \end{pmatrix} \otimes \hat{I}$  at the boundary positions. Panels (a1) and (a2) show the experimental and theoretical position distribution, respectively. Please note that we implement unitaries corresponding to up to 400 steps of the QW. Panel (a3) shows the coin-resolved probability distribution for the last step.

Fig. S3(b) shows a non-interacting QW on a line with periodic boundary conditions at positions  $\vec{x} = \pm 10$ . A non-interacting QW is realized by the transmission coin  $\hat{C}_T = \begin{pmatrix} 1 & 0 \\ 0 & 1 \end{pmatrix} \otimes \hat{I}$  at all positions. In addition, we implement periodic boundary conditions at the edges. These are interesting for, e.g., studying energy transport phenomena in biological samples since they allow for simulating ring structures (and really any closed graph). Again, panels (b1) and (b2) are the experimental and theoretical positions distributions, while panel (b3) is the coin resolved probability distribution for the last steps. For both case (a) and (b) we find a high mean similarity  $\bar{S} > 98\%$ .

### Grover walk on a cube

In the main manuscript, we presented the Grover walk on a four-dimensional hypercube, which is an essential building block for QW-based universal quantum computation. In Fig. S5, we study the unitaries associated with a QW on a cube. We prepared an input state  $|\psi\rangle = |\vec{x}=0\rangle \otimes \frac{1}{\sqrt{3}} \sum_{c=0}^2 |c\rangle$  that is, a state that is localised at the origin with a coin state that points equally in all three directions. This simply means that the walker will equally spread over the three neighbouring positions in the first step. Fig. S5 (a) and (b) show the experimental and theoretical position distribution, respectively. In contrast to the four-dimensional case from the main manuscript, we do not observe a revival of the walker at the origin within the first 34 steps. We do, however, observe that the walker localises at the other side of the cube after 23 steps. Panels (c) and (d) show the coin resolved probability distributions for the 23rd and 34th step, respectively. The transfer of the walker to the other side of the cube is clearly visible. In addition, the experiment reproduces the equal coin superposition well. In general, we again find a high mean similarity of  $\bar{S} > 98\%$ . We note that this study is not motivated by an important application, but was a good chance for trouble-shooting the experiment.

Fig. S6 investigates the same three-dimensional cube, but with a directed input state  $|\psi\rangle = |\vec{x}=0\rangle \otimes |c=0\rangle$  that is, a state that is localised at the origin and whose coin state points in only one direction. The panels are the same as for Fig. S5. In this case, we note the complete absence of a revival of the walker at any position. In contrast, as the walk continues, the walker becomes increasingly delocalised. For these measurements, we find a very high mean similarity of  $\bar{S} > 99\%$ . This supports a general trend: the more delocalized the walker, the better the performance of our approach. The reason for this is simple; a limited pulse

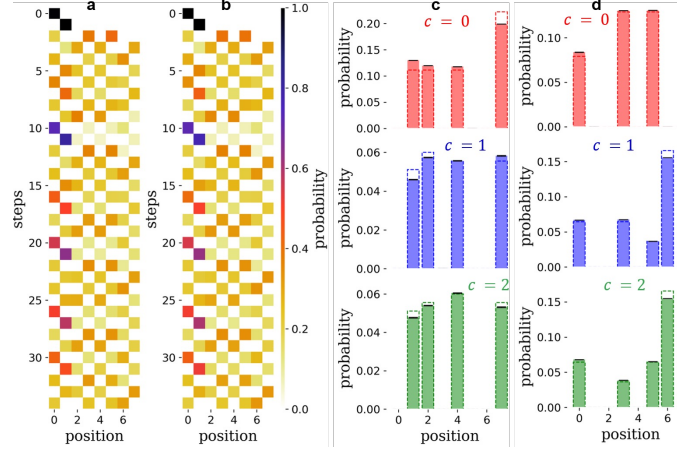

FIG. S6. Unitaries associated with a Grover walk on a cube with a directed input state. (a) Experimental position distribution. (b) Theoretical position distribution. (c) Coin-resolved probability distribution for the 23rd step. (d) Coin-resolved probability distribution for the 34th step. For more information, see the text.

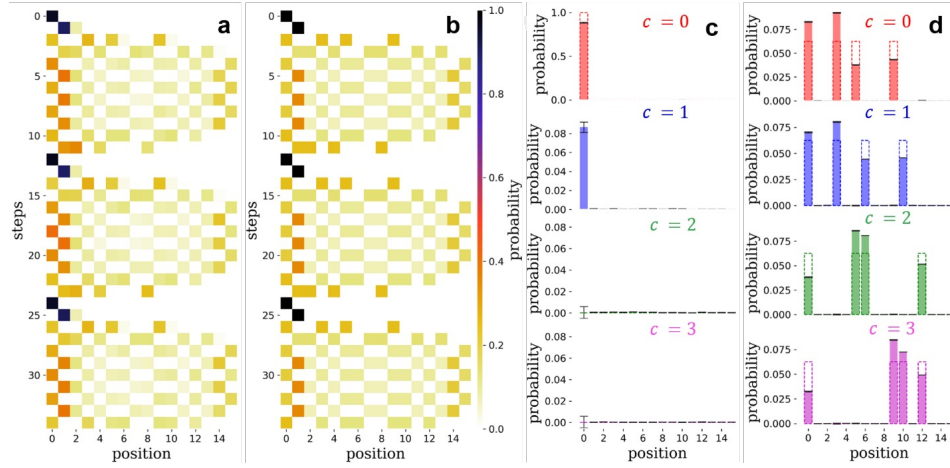

FIG. S7. Unitaries associated with a Grover walk on a four-dimensional hypercube with a directed input state  $|\psi\rangle = |\vec{x}=0\rangle \otimes |c=0\rangle$ . (a) Experimental position distribution. (b) Theoretical position distribution. (c) Coin-resolved probability distribution for the 12th step. (d) Coin-resolved probability distribution for the 34th step. For more information, see the text.

shaper resolution and finite phase matching bandwidth will introduce a constant small population of modes that are supposed to be empty. This has a more detrimental impact on a localised distribution than on a broad distribution.

### Grover walk on a hypercube

Finally, in Fig. S7, we present the results for unitaries pertinent to a QW on a four-dimensional hypercube with a directed input state  $|\psi\rangle = |\vec{x}=0\rangle \otimes |c=0\rangle$ , the same as above. This graph topology is the same as in the main manuscript, however with a different input state. Panels (a) and (b) show, again, the experimental and theoretical position distribution, respectively. As for the cube, we find that the walker takes a first step in a well-defined direction. Thereafter it delocalises and revives at the origin after 12 steps. We note that this behaviour, which was absent in the three-dimensional case, emerges again on the hypercube. Panel (c) shows the coin resolved probability distribution for the 12th step that is, at the first revival of the walker. Interestingly, the walker revives at the origin but with a different coin state compared to the initial state. Panel (d) shows the coin resolved probability distribution of the 34th step of the evolution. Again, we obtain a high mean similarity of  $\bar{S} > 98\%$ , similar to the other measurements presented in the Supplemental Material.

## IMPACT OF LIMITED MODE SELECTIVITY

In a real-world QPG, the mode selectivity is limited by the finite phase matching bandwidth. In fact, Eq. (4) describes an idealized situation. In a real system, we would rather perform a Schmidt decomposition of the transfer function, which reads

$$G(\omega_{\text{in}}, \omega_{\text{out}}) = \sum_{n=1}^N \sqrt{\lambda_n} f_n(\omega_{\text{in}}) g_n(\omega_{\text{out}}) \quad (22)$$

for a transfer function pertaining to an  $N$ -dimensional system. Here, we call the  $\sqrt{\lambda_n}$  the Schmidt coefficients and the  $f_n(\omega_{\text{in}})$  and  $g_n(\omega_{\text{out}})$  the Schmidt modes. For a normalized transfer function ( $\int d\omega_{\text{in}} d\omega_{\text{out}} |G(\omega_{\text{in}}, \omega_{\text{out}})|^2 = 1$ ), the Schmidt coefficients obey  $\sum_{n=1}^N \lambda_n = 1$ . In the case of an ideal QPG that addresses exactly one single input mode and transduces it to one single output mode,  $\sqrt{\lambda_1} = 1$  and  $\sqrt{\lambda_{>1}} = 0$ . Consequently, the transfer function reads

$$G(\omega_{\text{in}}, \omega_{\text{out}}) = \sum_{n=1}^N \sqrt{\lambda_n} f_n(\omega_{\text{in}}) g_n(\omega_{\text{out}}) = f_1(\omega_{\text{in}}) g_1(\omega_{\text{out}}), \quad (23)$$

which is exactly the result from Eq. (4). A non-perfect QPG features several Schmidt coefficients different from zero. In this case, we define a *modal selectivity*  $\kappa$  as

$$\kappa = \frac{\lambda_1}{\sum_{n=2}^N \lambda_n}. \quad (24)$$

Intuitively,  $\kappa$  quantifies the impact of undesired modes in the QPG operation. For a perfect QPG,  $\kappa \rightarrow \infty$ , as  $\sqrt{\lambda_{>1}} = 0$ . For a completely multimode QPG,  $\sqrt{\lambda_n} = 1/\sqrt{N}$  and hence  $\kappa = 1/(N-1) \leq 1$ . In other words, we want  $\kappa$  to be as large as possible.

In this work, we obtained typical values of  $\kappa \sim 200$ . This corresponds to a contribution of the dominating mode to the QPG operation of 99.5%. Loosely speaking, this number puts an upper bound on the performance of the QPG. A direct conversion to a maximum similarity is, however, not totally straightforward and heavily depends on the exact unitary. We note that better modal selectivities can be reached with a tighter spectral filtering of the output or a narrower phase matching function. Using the former method, we have seen values of  $\kappa \sim 500$ , which corresponds to a contribution of the dominant mode of 99.8%. The trade off is then modal selectivity and signal level and an optimum must be found for individual applications.

---

\* [benjamin.brecht@upb.de](mailto:benjamin.brecht@upb.de)
